# Supplementary material for: Exploiting Multimodal Reinforcement Learning for Simultaneous Machine Translation
Source: arXiv:2102.11387 source file (2021-02-22)
Supplement: Supplementary file 1 [file appendix.tex]

\phantom{foo}
